# Supplementary material for: Dr. GPT in Campus Counseling: Understanding Higher Education Students' Opinions on LLM-assisted Mental Health Services
Source: arXiv:2409.17572 source file (2024-09-26)
Supplement: Supplementary file 1 [file Appendix.tex]

\appendix

\section{Appendix}

\subsection{Protocol}

\section*{Introduction}
Good morning/afternoon! Thank you for joining us today. I’m [interviewer's name] from Princeton University.

This study aims to understand people’s opinions on LLM-assisted tools when used by mental health professionals. We will take the next 60 minutes to conduct an interview based on some imaginary scenarios. The interview is semi-structured; we plan to ask questions covering the following aspects but may omit some or add some follow-up questions based on your answers.

There are no right or wrong answers; what we are interested in is your opinions on these scenarios.

\section*{Consent and Participation}
If there is anything you'd prefer not to answer or discuss please let us know. If you need anything or wish to pause the interview also feel free to let us know. In the survey we obtained your consent to be the subject of the research and also to record the session for research purposes only.

After this interview we will send you a 15-dollar gift card as a token of our appreciation for your participation.

Do you have any questions regarding this interview? [pause for answer] If not we will start recording and begin the interview. Would you mind recording this interview for research purposes? [pause for answer]

[start recording]
\subsection{Scenarios \& Questions}

% \section*{Scenarios \& Questions}

\subsection*{Scenario 1: General Information Inquiry}

\textbf{Scenario Summary:}
Alex, a sophomore who's been struggling with one advanced level class. Alex was a straight-A student before. But now Alex is afraid that he might fail one class and have a bad grade in the college transcript further having a negative consequence in his future grad applications. Alex cannot stop thinking about this. He does not want to eat, talk, and sleep. He doesn’t know why.

Therefore, Alex told LLM he is worrying about his grades and does not want to eat and sleep. He asked LLM what are the professional terms for these symptoms and how he should deal with them and if there are any supporting resources. The platform offers a variety of resources from articles to webinars and helpline numbers, providing Alex with a comprehensive understanding.

\textbf{Probing question:}
Alex has little knowledge about mental health. How effective do you believe LLM tools like ChatGPT can be in introducing individuals about mental health? What disadvantages do you see with relying on AI for this?

\subsection*{Scenario 2: Initial Screening}

\textbf{Scenario Summary:}
Chris, a junior, heavily relies on technology for daily activities, including mental health management. Chris uses an LLM tool for daily mental health check-ins and advice. This dependence raises concerns about over-reliance on technology for emotional well-being.

\textbf{Probing question:}
In your opinion, what are the potential risks of depending too much on technology, like LLM tools, for managing one's mental health?

\subsection*{Scenario 3: Reshaping Patient-Expert Dynamics}

\textbf{Scenario Summary:}
Taylor, a graduate student, regularly consults a therapist. Recently, Taylor's therapist started using an LLM tool to supplement their sessions. This change brings up questions about the role of AI in the patient-therapist relationship.

\textbf{Probing question:}
How do you think the introduction of LLM tools in therapy sessions might affect the dynamics between a patient and a mental health expert?

\subsection*{Scenario 4: Long-term Care}

\textbf{Scenario Summary:}
Jordan, dealing with anxiety, uses an LLM-based app that incorporates user feedback to improve its responses. This scenario explores the effectiveness of such feedback mechanisms.

\textbf{Probing question:}
How important do you think a feedback mechanism is in LLM-based mental health tools? Can you think of ways this could be beneficial or detrimental?

\subsection*{Scenario 5: Follow-up Care}

\textbf{Scenario Summary:}
Sam, who has been using an LLM tool for mental health support, moves to a new city and has to find a new therapist. The scenario discusses the role of LLM tools in ensuring continuity of care during such transitions.

\textbf{Probing question:}
What role do you think LLM tools can play in maintaining continuity of care when a person like Sam moves to a new location or changes therapists?
